# Supplementary material for: A fast method to estimate speciation parameters in a model of isolation with an initial period of gene flow and to test alternative evolutionary scenarios
Source: arXiv:1511.05478 ancillary file (2015-11-17)
Supplement: Supplementary file 1 [file Supplementary_Material.pdf]

## Supplementary Material

We used R (R Development Core Team, 2011) to implement our method. Here we provide our code to obtain ML estimates under the IIM model, for the case where all loci have the same mutation rate, and for the case where different loci have different mutation rates. After entering the data as described, the remaining code can simply be pasted into an R document (R will automatically ignore the comments included); the starting values for the minimization of the negated loglikelihood may need to be adjusted to values that are broadly reasonable for the specific data set to be analyzed. We also provide our R code for simulating pairwise difference data under the IIM model. The code below uses the results of Wilkinson-Herbots (2012) for the IIM model, and those of Takahata et al. (1995) for the isolation model (see also Wilkinson-Herbots 2008). A simplified version of the code which obtains ML estimates under a symmetric IM model (based on the results in Wilkinson-Herbots 2008) is available from the author upon request.

1. **R code to fit an IIM model to pairwise difference data where all loci have the same mutation rate:**

   **(a) if pairwise difference data are available between species and within one of the species:**

```
# input required:
# k11: vector containing the different observed values of the number of pairwise differences within species 1
# freq11: vector containing the observed frequencies of the values in k11
# k12: vector containing the different observed values of the number of pairwise differences between the two species
# freq12: vector containing the observed frequencies of the values in k12
#
# for example, for the trimmed version of Drosophila "data set 3" described in "Materials and Methods"
# (data from Wang and Hey 2010, trimmed according to Lohse et al. 2011):
# D.simulans - D.simulans pairwise differences:
k11 <- c(0,1,2,3,4,5,6,7,8,9,10,11,12,13,14,15,16,17,18,19,20,21,23,26)
freq11 <- c(3504,1809,1398,996,637,397,267,156,71,65,24,18,10,12,2,4,6,2,1,3,1,1,1,1)
# D.simulans - D.melanogaster pairwise differences:
k12 <- c(0,1,2,3,4,5,6,7,8,9,10,11,12,13,14,15,16,17,18,19,20,21,22,24,25,27,31)
freq12 <- c(118,413,912,1604,2061,2493,2524,2411,1970,1472,1076,665,460,244,156,71,49,31,20,8,5,2,2,1,1,1,1)

# ML estimates are obtained for the reparameterized IIM model - see equation (4) in the main text;
# a complete isolation model is fitted first in order to provide reasonable starting values for the IIM model
# (this step may be omitted if good enough starting values can be guessed):

# calculation of negated loglikelihood for the reparameterized isolation model :
negll.isolation<- function(x){

   T <- x[1]
   theta <- x[2]
   theta.a <- x[3]

   l11 <- log( (theta^k11/(1+theta)^(k11+1))*(1-ppois(k11,(1/theta+1)*T,log.p=FALSE))
           +((theta.a)^k11/(1+theta.a)^(k11+1))*exp((1/theta.a - 1/theta)*T)*ppois(k11,(1/theta.a+1)*T,log.p=FALSE) )

   l12 <- k12*log(theta.a)-(k12+1)*log(1+theta.a)+T/theta.a + ppois(k12,(1/theta.a + 1)*T,log.p=TRUE)

   -sum(l11*freq11)-sum(l12*freq12)
}

# to obtain parameter estimates for the reparameterized isolation model (if this doesn't work, try different starting values):
isolation <- nlminb(c(1,0.5,0.5),negll.isolation,control=list(eval.max=10000,iter.max=10000,abs.tol= 1e-20,step.min=0.1,
                    step.max=10),lower=rep(0,3))
# parameter estimates:
isolation.estimates <- isolation$par
# maximized loglikelihood:
isolation.maxll <-  -isolation$objective
# AIC score:
isolation.AIC <- (-isolation.maxll+3)*2

# to obtain standard errors (warnings may result from nlm trying negative parameter values – for our purposes these can be ignored):
isolation2 <- nlm(negll.isolation,isolation$par,hessian=TRUE)
isolation.VC <- solve(isolation2$hessian)
isolation.se <- sqrt(diag(isolation.VC))
```

```
# calculation of negated loglikelihood for the reparameterized IIM model:
negll.IIM <- function(x){

   T1 <- x[1]
   V <- x[2]
   theta1<- x[3]
   theta<- x[4]
   theta.a<- x[5]
   M <- x[6]

   T0 <- T1+V
   D <- 4*M^2+1
   L1 <- (2*M+1-sqrt(D))/2
   L2 <- (2*M+1+sqrt(D))/2
   A01 <- (L2-1)/(L2-L1)
   A02 <- (1-L1)/(L2-L1)
   A11 <- L2/(L2-L1)
   A12 <- -L1/(L2-L1)
   R1 <- L1/theta
   R2 <- L2/theta

   l11 <- log( (theta1^k11/(1+theta1)^(k11+1))*(1-ppois(k11,(1/theta1 +1)*T1,log.p=FALSE))
            +exp(-T1/theta1)*( A01*R1*exp(R1*T1)*(ppois(k11,(R1+1)*T1,log.p=FALSE)
            -ppois(k11,(R1+1)*T0,log.p=FALSE))/(R1+1)^(k11+1)
            +A02*R2*exp(R2*T1)*(ppois(k11,(R2+1)*T1,log.p=FALSE)-ppois(k11,(R2+1)*T0,log.p=FALSE))/(R2+1)^(k11+1)
            +((theta.a)^k11/(1+theta.a)^(k11+1))*exp(T0/theta.a)*ppois(k11,(1/theta.a + 1)*T0,log.p=FALSE)
            *(A01*exp(-R1*V)+A02*exp(-R2*V)) ) )

   l12 <- log( A11*R1*exp(R1*T1)*(ppois(k12,(R1+1)*T1,log.p=FALSE)-ppois(k12,(R1+1)*T0,log.p=FALSE))/(R1+1)^(k12+1)
            +A12*R2*exp(R2*T1)*(ppois(k12,(R2+1)*T1,log.p=FALSE)-ppois(k12,(R2+1)*T0,log.p=FALSE))/(R2+1)^(k12+1)
            +((theta.a)^k12/(1+theta.a)^(k12+1))*exp(T0/theta.a)*ppois(k12,(1/theta.a + 1)*T0,log.p=FALSE)
            *(A11*exp(-R1*V)+A12*exp(-R2*V)) )

   -sum(l11*freq11)-sum(l12*freq12)
}

# to obtain parameter estimates for the reparameterized IIM model (if this doesn't work, try different starting values):
IIM <- nlminb(c(isolation$par[1]/2,isolation$par[1]/2, isolation$par[2],(isolation$par[2]+isolation$par[3]/2)/2,isolation$par[3],0.5),
          negll.IIM,control=list(eval.max=10000,iter.max=10000,abs.tol= 1e-20,step.min=0.1,step.max=10),lower=rep(0,6))
# parameter estimates:
IIM.estimates <- IIM$par
# maximized loglikelihood:
IIM.maxll <- -IIM$objective
# AIC score:
IIM.AIC <- (-IIM.maxll+6)*2

# to obtain standard errors (warnings may result from nlm trying negative parameter values – for our purposes these can be ignored):
IIM2 <- nlm(negll.IIM,IIM$par,hessian=TRUE)
IIM.VC <- solve(IIM2$hessian)
IIM.se <- sqrt(diag(IIM.VC))
# Note: this calculation of standard errors will not work if one or more parameters (for example, M) are estimated to be zero;
# in that case a simplified model can be fitted, removing the zero parameter(s) from the model, and estimated standard errors for the
# remaining parameters can then be computed as above under the reduced model.

# results:
# IIM.estimates = the ML estimates for (T1, V, θ1, θ, θa, M) in the reparameterized IIM model;
# IIM.se = the estimated standard errors of these parameter estimates;
# IIM .maxll = the maximized loglikelihood for the IIM model;
# IIM.AIC = the AIC score of the IIM model.
# isolation.estimates = the ML estimates for (T,θ, θa) in the reparameterized isolation model;
# isolation.se = the estimated standard errors of these parameter estimates;
# isolation.maxll = the maximized loglikelihood for the isolation model;
# isolation.AIC = the AIC score of the isolation model.
```

```
# to display the results:
cat("\n","IIM model:", "\n",
"ML estimate for (T_1, V, θ_1, θ, θ_a, M):",IIM.estimates,"\n",
"estimated s.e. for (T_1, V, θ_1, θ, θ_a, M):",IIM.se,"\n",
"maximized loglikelihood =",IIM.maxll,"\n",
"AIC score =",IIM.AIC,"\n","\n",
"isolation model:", "\n",
"ML estimate for (T, θ, θ_a):",isolation.estimates,"\n",
"estimated s.e. for (T, θ, θ_a):",isolation.se,"\n",
"maximized loglikelihood =",isolation.maxll,"\n",
"AIC score =",isolation.AIC,"\n")
```

**(b) if pairwise difference data are available between species and within both species:**

```
# input required (see 1.(a) above for an example):
k11 <-  # input vector containing the different observed values of the number of pairwise differences within species 1
freq11 <-  # input vector containing the observed frequencies of the values in k11
k22 <-  # input vector containing the different observed values of the number of pairwise differences within species 2
freq22  <-  # input vector containing the observed frequencies of the values in k22
k12 <-  # input vector containing the different observed values of the number of pairwise differences between the two species
freq12 <-  # input vector containing the observed frequencies of the values in k12

# ML estimates are obtained for the reparameterized IIM model - see equation (4) in the main text;
# a complete isolation model is fitted first in order to provide reasonable starting values for the IIM model
# (this step may be omitted if good enough starting values can be guessed):

# calculation of negated loglikelihood for the reparameterized isolation model :
negll.isolation<- function(x){

   T <- x[1]
   theta1 <- x[2]
   theta2 <- x[3]
   theta.a <- x[4]

   l11 <- log( (theta1^k11/(1+theta1)^(k11+1))*(1-ppois(k11,(1/theta1+1)*T,log.p=FALSE))
            +((theta.a)^k11/(1+theta.a)^(k11+1))*exp((1/theta.a - 1/theta1)*T)*ppois(k11,(1/theta.a+1)*T,log.p=FALSE) )

   l22 <- log( (theta2^k22/(1+theta2)^(k22+1))*(1-ppois(k22,(1/theta2+1)*T,log.p=FALSE))
            +((theta.a)^k22/(1+theta.a)^(k22+1))*exp((1/theta.a - 1/theta2)*T)*ppois(k22,(1/theta.a+1)*T,log.p=FALSE) )

   l12 <- k12*log(theta.a)-(k12+1)*log(1+theta.a)+T/theta.a + ppois(k12,(1/theta.a + 1)*T,log.p=TRUE)

   -sum(l11*freq11)-sum(l22*freq22)-sum(l12*freq12)
}

# to obtain parameter estimates for the reparameterized isolation model (if this doesn't work, try different starting values):
isolation <- nlminb(c(1,0.5,0.5,0.5),negll.isolation,control=list(eval.max=10000,iter.max=10000,abs.tol= 1e-20,step.min=0.1,
                  step.max=10),lower=rep(0,4))
# parameter estimates:
isolation.estimates <- isolation$par
# maximized loglikelihood:
isolation.maxll <- -isolation$objective
# AIC score:
isolation.AIC <- (-isolation.maxll+4)*2

# to obtain standard errors (warnings may result from nlm trying negative parameter values – for our purposes these can be ignored):
isolation2 <- nlm(negll.isolation,isolation$par,hessian=TRUE)
isolation.VC <- solve(isolation2$hessian)
isolation.se <- sqrt(diag(isolation.VC))
```

```
# calculation of negated loglikelihood for the reparameterized IIM model :
negll.IIM <- function(x){

   T1 <- x[1]
   V <- x[2]
   theta1 <- x[3]
   theta2 <- x[4]
   theta <- x[5]
   theta.a <- x[6]
   M <- x[7]

   T0 <- T1+V
   D <- 4*M^2+1
   L1 <- (2*M+1-sqrt(D))/2
   L2 <- (2*M+1+sqrt(D))/2
   A01 <- (L2-1)/(L2-L1)
   A02 <- (1-L1)/(L2-L1)
   A11 <- L2/(L2-L1)
   A12 <- -L1/(L2-L1)
   R1 <- L1/theta
   R2 <- L2/theta

   l11 <- log( (theta1^k11/(1+theta1)^(k11+1))*(1-ppois(k11,(1/theta1 +1)*T1,log.p=FALSE))
           +exp(-T1/theta1)*( A01*R1*exp(R1*T1)*(ppois(k11,(R1+1)*T1,log.p=FALSE)
           -ppois(k11,(R1+1)*T0,log.p=FALSE))/(R1+1)^(k11+1)
           +A02*R2*exp(R2*T1)*(ppois(k11,(R2+1)*T1,log.p=FALSE)-ppois(k11,(R2+1)*T0,log.p=FALSE))/(R2+1)^(k11+1)
           +((theta.a)^k11/(1+theta.a)^(k11+1))*exp(T0/theta.a)*ppois(k11,(1/theta.a + 1)*T0,log.p=FALSE)
           *(A01*exp(-R1*V)+A02*exp(-R2*V)) ) )

   l22 <- log( (theta2^k22/(1+theta2)^(k22+1))*(1-ppois(k22,(1/theta2 +1)*T1,log.p=FALSE))
           +exp(-T1/theta2)*( A01*R1*exp(R1*T1)*(ppois(k22,(R1+1)*T1,log.p=FALSE)
           -ppois(k22,(R1+1)*T0,log.p=FALSE))/(R1+1)^(k22+1)
           +A02*R2*exp(R2*T1)*(ppois(k22,(R2+1)*T1,log.p=FALSE)-ppois(k22,(R2+1)*T0,log.p=FALSE))/(R2+1)^(k22+1)
           +((theta.a)^k22/(1+theta.a)^(k22+1))*exp(T0/theta.a)*ppois(k22,(1/theta.a + 1)*T0,log.p=FALSE)
           *(A01*exp(-R1*V)+A02*exp(-R2*V)) ) )

   l12 <- log( A11*R1*exp(R1*T1)*(ppois(k12,(R1+1)*T1,log.p=FALSE)-ppois(k12,(R1+1)*T0,log.p=FALSE))/(R1+1)^(k12+1)
           +A12*R2*exp(R2*T1)*(ppois(k12,(R2+1)*T1,log.p=FALSE)-ppois(k12,(R2+1)*T0,log.p=FALSE))/(R2+1)^(k12+1)
           +((theta.a)^k12/(1+theta.a)^(k12+1))*exp(T0/theta.a)*ppois(k12,(1/theta.a + 1)*T0,log.p=FALSE)
           *(A11*exp(-R1*V)+A12*exp(-R2*V)) )

   -sum(l11*freq11) -sum(l22*freq22)-sum(l12*freq12)
}

# to obtain parameter estimates for the reparameterized IIM model (if this doesn't work, try different starting values):
IIM <- nlminb(c(isolation$par[1]/2,isolation$par[1]/2, isolation$par[2], isolation$par[3],
          (isolation$par[2]+isolation$par[3]+isolation$par[4])/4,isolation$par[4],0.5),negll.IIM,
          control=list(eval.max=10000,iter.max=10000,abs.tol= 1e-20,step.min=0.1,step.max=10),lower=rep(0,7))
# parameter estimates:
IIM.estimates<- IIM$par
# maximized loglikelihood:
IIM.maxll<- -IIM$objective
# AIC score:
IIM.AIC <- (-IIM.maxll+7)*2

# to obtain standard errors (warnings may result from nlm trying negative parameter values – for our purposes these can be ignored):
IIM2<-nlm(negll.IIM,IIM$par,hessian=TRUE)
IIM.VC<-solve(IIM2$hessian)
IIM.se<-sqrt(diag(IIM.VC))
# Note: this calculation of standard errors will not work if one or more parameters (for example, M) are estimated to be zero;
# in that case a simplified model can be fitted, removing the zero parameter(s) from the model, and estimated standard errors for the
# remaining parameters can then be computed as above under the reduced model.
```

```
# results:
# IIM.estimates = the ML estimates for (T_1, V, θ_1, θ_2, θ, θ_a, M) in the reparameterized IIM model;
# IIM.se = the estimated standard errors of these parameter estimates;
# IIM .maxll = the maximized loglikelihood for the IIM model;
# IIM.AIC = the AIC score of the IIM model.
# isolation.estimates = the ML estimates for (T, θ_1, θ_2, θ_a) in the reparameterized isolation model;
# isolation.se = the estimated standard errors of these parameter estimates;
# isolation.maxll = the maximized loglikelihood for the isolation model;
# isolation.AIC = the AIC score of the isolation model.

# to display the results:
cat("\n","IIM model:", "\n",
"ML estimate for (T_1, V, θ_1, θ_2, θ, θ_a, M):",IIM.estimates,"\n",
"estimated s.e. for (T_1, V, θ_1, θ_2, θ, θ_a, M):",IIM.se,"\n",
"maximized loglikelihood =",IIM.maxll,"\n",
"AIC score =",IIM.AIC,"\n","\n",
"isolation model:", "\n",
"ML estimate for (T, θ_1, θ_2, θ_a):",isolation.estimates,"\n",
"estimated s.e. for (T, θ_1, θ_2, θ_a):",isolation.se,"\n",
"maximized loglikelihood =",isolation.maxll,"\n",
"AIC score =",isolation.AIC,"\n")
```

## 2. R code to fit an IIM model to pairwise difference data where different loci have different mutation rates:

### (a) if pairwise difference data are available between species and within one of the species:

```
# input required: vectors of within- and between-species pairwise differences, and the relative mutation rates of the loci concerned:
k11 <-  # input vector containing the numbers of nucleotide differences between pairs of sequences from species 1
        # (this vector should contain one entry for each locus at which two sequences from species 1 are compared)
k12 <-  # input vector containing the numbers of nucleotide differences between pairs of sequences from different species
        # (this vector should contain one entry for each locus at which two sequences from different species are compared)
# for example, for Drosophila "data set 3" described in "Materials and Methods" (30,247 loci in total, from Wang and Hey 2010):
# k11 is a vector of length 10,083 containing D.simulans-D.simulans numbers of pairwise differences;
# k12 is a vector of length 20,164 containing D.simulans-D.melanogaster numbers of pairwise differences.
r11 <-  # input vector containing the relative mutation rate (or the outgroup divergence) of each of the loci in k11;
        # (this vector should contain one entry for each locus at which two sequences from species 1 are compared;
        # all entries of r11 must be > 0)
r12 <-  # input vector containing the relative mutation rate (or the outgroup divergence) of each of the loci in k12
        # (this vector should contain one entry for each locus at which two sequences from different species are compared;
        # all entries of r12 must be > 0)

# we scale the relative mutation rates so that their average over all the loci included in the analysis is 1:
r.average <- mean(c(r11,r12))
r11 <- r11/r.average
r12 <- r12/r.average

# ML estimates are obtained for the reparameterized IIM model - see equation (4) in the main text,
# where θ is now the average scaled mutation rate over all the loci included in the analysis.
# A complete isolation model is fitted first in order to provide reasonable starting values for the IIM model
# (this step may be omitted if good enough starting values can be guessed).

# calculation of negated loglikelihood for the reparameterized isolation model :
negll.isolation<- function(x){

  T.average <- x[1]
  theta.average <- x[2]
  theta.a.average <- x[3]
```

```
    T <- T.average*r11
    theta <- theta.average*r11
    theta.a <- theta.a.average*r11
    l11 <- log( (theta^k11/(1+theta)^(k11+1))*(1-ppois(k11,(1/theta+1)*T,log.p=FALSE))
              +((theta.a)^k11/(1+theta.a)^(k11+1))*exp((1/theta.a - 1/theta)*T)*ppois(k11,(1/theta.a+1)*T,log.p=FALSE) )

    T <- T.average*r12
    theta.a <- theta.a.average*r12
    l12 <- k12*log(theta.a)-(k12+1)*log(1+theta.a)+T/theta.a + ppois(k12,(1/theta.a + 1)*T,log.p=TRUE)

    -sum(l11)-sum(l12)
}

# to obtain parameter estimates for the reparameterized isolation model (if this doesn't work, try different starting values):
isolation <- nlminb(c(10,5,5),negll.isolation,control=list(eval.max=10000,iter.max=10000,abs.tol= 1e-20,step.min=0.1,step.max=10),
                lower=rep(0,3))
# parameter estimates:
isolation.estimates <- isolation$par
# maximized loglikelihood:
isolation.maxll <- -isolation$objective
# AIC score:
isolation.AIC <- (-isolation.maxll+3)*2

# to obtain standard errors (warnings may result from nlm trying negative parameter values – for our purposes these can be ignored):
isolation2 <- nlm(negll.isolation,isolation$par,hessian=TRUE)
isolation.VC <- solve(isolation2$hessian)
isolation.se <- sqrt(diag(isolation.VC))


# calculation of negated loglikelihood for the reparameterized IIM model :
negll.IIM <- function(x){

    T1.average <- x[1]
    V.average<- x[2]
    theta1.average <- x[3]
    theta.average<- x[4]
    theta.a.average<- x[5]
    M <- x[6]

    D <- 4*M^2+1
    L1 <- (2*M+1-sqrt(D))/2
    L2 <- (2*M+1+sqrt(D))/2
    A01 <- (L2-1)/(L2-L1)
    A02 <- (1-L1)/(L2-L1)
    A11 <- L2/(L2-L1)
    A12 <- -L1/(L2-L1)
    R1.average <- L1/theta.average
    R2.average <- L2/theta.average

    T1 <- T1.average*r11
    V <- V.average*r11
    T0 <- T1+V
    theta1 <- theta1.average*r11
    theta.a <- theta.a.average*r11
    R1 <- R1.average/r11
    R2 <- R2.average/r11
    l11 <- log( (theta1^k11/(1+theta1)^(k11+1))*(1-ppois(k11,(1/theta1 +1)*T1,log.p=FALSE))+exp(-T1/theta1)
              *( A01*R1*exp(R1*T1)*(ppois(k11,(R1+1)*T1,log.p=FALSE)-ppois(k11,(R1+1)*T0,log.p=FALSE))/(R1+1)^(k11+1)
              +A02*R2*exp(R2*T1)*(ppois(k11,(R2+1)*T1,log.p=FALSE)-ppois(k11,(R2+1)*T0,log.p=FALSE))/(R2+1)^(k11+1)
              +((theta.a)^k11/(1+theta.a)^(k11+1))*exp(T0/theta.a)*ppois(k11,(1/theta.a + 1)*T0,log.p=FALSE)
              *(A01*exp(-R1*V)+A02*exp(-R2*V)) ) )
```

```
  T1 <- T1.average*r12
  V <- V.average*r12
  T0 <- T1+V
  theta.a <- theta.a.average*r12
  R1 <- R1.average/r12
  R2 <- R2.average/r12
  l12 <- log( A11*R1*exp(R1*T1)*(ppois(k12,(R1+1)*T1,log.p=FALSE)-ppois(k12,(R1+1)*T0,log.p=FALSE))/(R1+1)^(k12+1)
        +A12*R2*exp(R2*T1)*(ppois(k12,(R2+1)*T1,log.p=FALSE)-ppois(k12,(R2+1)*T0,log.p=FALSE))/(R2+1)^(k12+1)
        +((theta.a)^k12/(1+theta.a)^(k12+1))*exp(T0/theta.a)*ppois(k12,(1/theta.a + 1)*T0,log.p=FALSE)
        *(A11*exp(-R1*V)+A12*exp(-R2*V)) )

  -sum(l11)-sum(l12)
}

# to obtain parameter estimates for the reparameterized IIM model (if this doesn't work, try different starting values):
IIM <- nlminb(c(isolation$par[1]/2,isolation$par[1]/2, isolation$par[2],(isolation$par[2]+isolation$par[3]/2)/2,isolation$par[3],0.5),
       negll.IIM,control=list(eval.max=10000,iter.max=10000,abs.tol= 1e-20,step.min=0.1,step.max=10),lower=rep(0,6))
# parameter estimates:
IIM.estimates <- IIM$par
# maximized loglikelihood:
IIM.maxll <- -IIM$objective
# AIC score:
IIM.AIC <- (-IIM.maxll+6)*2

# to obtain standard errors (warnings may result from nlm trying negative parameter values – for our purposes these can be ignored):
IIM2 <- nlm(negll.IIM,IIM$par,hessian=TRUE)
IIM.VC <- solve(IIM2$hessian)
IIM.se <- sqrt(diag(IIM.VC))
# Note: this calculation of standard errors will not work if one or more parameters (for example, M) are estimated to be zero;
# in that case a simplified model can be fitted, removing the zero parameter(s) from the model, and estimated standard errors for the
# remaining parameters can then be computed as above under the reduced model.

# results:
# IIM.estimates = the ML estimates for (T_1, V, θ_1, θ, θ_a, M) in the reparameterized IIM model;
# IIM.se = the estimated standard errors of these parameter estimates;
# IIM .maxll = the maximized loglikelihood for the IIM model;
# IIM.AIC = the AIC score of the IIM model.
# isolation.estimates = the ML estimates for (T,θ, θ_a) in the reparameterized isolation model;
# isolation.se = the estimated standard errors of these parameter estimates;
# isolation.maxll = the maximized loglikelihood for the isolation model;
# isolation.AIC = the AIC score of the isolation model.

# to display the results:
cat("\n","IIM model:", "\n",
"ML estimate for (T_1, V, θ_1, θ, θ_a, M):",IIM.estimates,"\n",
"estimated s.e. for (T_1, V, θ_1, θ, θ_a, M):",IIM.se,"\n",
"maximized loglikelihood =",IIM.maxll,"\n",
"AIC score =",IIM.AIC,"\n","\n",
"isolation model:", "\n",
"ML estimate for (T, θ, θ_a):",isolation.estimates,"\n",
"estimated s.e. for (T, θ, θ_a):",isolation.se,"\n",
"maximized loglikelihood =",isolation.maxll,"\n",
"AIC score =",isolation.AIC,"\n")
```

**(b) if pairwise difference data are available between species and within both species:**

```
# input required: vectors of within- and between-species pairwise differences, and the relative mutation rates of the loci concerned:
k11 <-  # input vector containing the numbers of nucleotide differences between pairs of sequences from species 1
        # (this vector should contain one entry for each locus at which two sequences from species 1 are compared)
k22 <-  # input vector containing the numbers of nucleotide differences between pairs of sequences from species 2
        # (this vector should contain one entry for each locus at which two sequences from species 2 are compared)
k12 <-  # input vector containing the numbers of nucleotide differences between pairs of sequences from different species
        # (this vector should contain one entry for each locus at which two sequences from different species are compared)
```

```
r11 <-  # input vector containing the relative mutation rate (or the outgroup divergence) of each of the loci in k11
        # (this vector should contain one entry for each locus at which two sequences from species 1 are compared;
        # all entries of r11 must be > 0)
r22 <-  # input vector containing the relative mutation rate (or the outgroup divergence) of each of the loci in k22
        # (this vector should contain one entry for each locus at which two sequences from species 2 are compared;
        # all entries of r22 must be > 0)
r12 <-  # input vector containing the relative mutation rate (or the outgroup divergence) of each of the loci in k12
        # (this vector should contain one entry for each locus at which two sequences from different species are compared;
        # all entries of r12 must be > 0)

# we scale the relative mutation rates so that their average over all the loci included in the analysis is 1:
r.average <- mean(c(r11,r22,r12))
r11 <- r11/r.average
r22 <- r22/r.average
r12 <- r12/r.average

# ML estimates are obtained for the reparameterized IIM model - see equation (4) in the main text,
# where θ is now the average scaled mutation rate over all the loci included in the analysis.
# A complete isolation model is fitted first in order to provide reasonable starting values for the IIM model
# (this step may be omitted if good enough starting values can be guessed).

# calculation of negated loglikelihood for the reparameterized isolation model :
negll.isolation <- function(x){

  T.average <- x[1]
  theta1.average <- x[2]
  theta2.average <- x[3]
  theta.a.average <- x[4]

  T <- T.average*r11
  theta1 <- theta1.average*r11
  theta.a <- theta.a.average*r11
  l11 <- log( (theta1^k11/(1+theta1)^(k11+1))*(1-ppois(k11,(1/theta1+1)*T,log.p=FALSE))
        +((theta.a)^k11/(1+theta.a)^(k11+1))*exp((1/theta.a - 1/theta1)*T)*ppois(k11,(1/theta.a+1)*T,log.p=FALSE) )

  T <- T.average*r22
  theta2 <- theta2.average*r22
  theta.a <- theta.a.average*r22
  l22 <- log( (theta2^k22/(1+theta2)^(k22+1))*(1-ppois(k22,(1/theta2+1)*T,log.p=FALSE))
        +((theta.a)^k22/(1+theta.a)^(k22+1))*exp((1/theta.a - 1/theta2)*T)*ppois(k22,(1/theta.a+1)*T,log.p=FALSE) )

  T <- T.average*r12
  theta.a <- theta.a.average*r12
  l12 <- k12*log(theta.a)-(k12+1)*log(1+theta.a)+T/theta.a + ppois(k12,(1/theta.a + 1)*T,log.p=TRUE)

  -sum(l11)-sum(l22)-sum(l12)
}

# to obtain parameter estimates for the reparameterized isolation model (if this doesn't work, try different starting values):
isolation <- nlminb(c(10,5,5,5),negll.isolation,control=list(eval.max=10000,iter.max=10000,abs.tol= 1e-20,step.min=0.1,
            step.max=10),lower=rep(0,4))
# parameter estimates:
isolation.estimates <- isolation$par
# maximized loglikelihood:
isolation.maxll <- -isolation$objective
# AIC score:
isolation.AIC <- (-isolation.maxll+4)*2

# to obtain standard errors (warnings may result from nlm trying negative parameter values – for our purposes these can be ignored):
isolation2 <- nlm(negll.isolation,isolation$par,hessian=TRUE)
isolation.VC <- solve(isolation2$hessian)
isolation.se <- sqrt(diag(isolation.VC))
```

# calculation of negated loglikelihood for the reparameterized IIM model :

```
negll.IIM <- function(x){

   T1.average <- x[1]
   V.average <- x[2]
   theta1.average <- x[3]
   theta2.average <- x[4]
   theta.average <- x[5]
   theta.a.average <- x[6]
   M <- x[7]

   D <- 4*M^2+1
   L1 <- (2*M+1-sqrt(D))/2
   L2 <- (2*M+1+sqrt(D))/2
   A01 <- (L2-1)/(L2-L1)
   A02 <- (1-L1)/(L2-L1)
   A11 <- L2/(L2-L1)
   A12 <- -L1/(L2-L1)
   R1.average <- L1/theta.average
   R2.average <- L2/theta.average


   T1 <- T1.average*r11
   V <- V.average*r11
   T0 <- T1+V
   theta1 <- theta1.average*r11
   theta.a <- theta.a.average*r11
   R1 <- R1.average/r11
   R2 <- R2.average/r11
   l11 <- log( (theta1^k11/(1+theta1)^(k11+1))*(1-ppois(k11,(1/theta1 +1)*T1,log.p=FALSE))+exp(-T1/theta1)
           *( A01*R1*exp(R1*T1)*(ppois(k11,(R1+1)*T1,log.p=FALSE)-ppois(k11,(R1+1)*T0,log.p=FALSE))/(R1+1)^(k11+1)
           +A02*R2*exp(R2*T1)*(ppois(k11,(R2+1)*T1,log.p=FALSE)-ppois(k11,(R2+1)*T0,log.p=FALSE))/(R2+1)^(k11+1)
           +((theta.a)^k11/(1+theta.a)^(k11+1))*exp(T0/theta.a)*ppois(k11,(1/theta.a + 1)*T0,log.p=FALSE)
           *(A01*exp(-R1*V)+A02*exp(-R2*V)) ) )

   T1 <- T1.average*r22
   V <- V.average*r22
   T0 <- T1+V
   theta2 <- theta2.average*r22
   theta.a <- theta.a.average*r22
   R1 <- R1.average/r22
   R2 <- R2.average/r22
   l22 <- log( (theta2^k22/(1+theta2)^(k22+1))*(1-ppois(k22,(1/theta2 +1)*T1,log.p=FALSE))+exp(-T1/theta2)
           *( A01*R1*exp(R1*T1)*(ppois(k22,(R1+1)*T1,log.p=FALSE)-ppois(k22,(R1+1)*T0,log.p=FALSE))/(R1+1)^(k22+1)
           +A02*R2*exp(R2*T1)*(ppois(k22,(R2+1)*T1,log.p=FALSE)-ppois(k22,(R2+1)*T0,log.p=FALSE))/(R2+1)^(k22+1)
           +((theta.a)^k22/(1+theta.a)^(k22+1))*exp(T0/theta.a)*ppois(k22,(1/theta.a + 1)*T0,log.p=FALSE)
           *(A01*exp(-R1*V)+A02*exp(-R2*V)) ) )

   T1 <- T1.average*r12
   V <- V.average*r12
   T0 <- T1+V
   theta.a <- theta.a.average*r12
   R1 <- R1.average/r12
   R2 <- R2.average/r12
   l12 <- log( A11*R1*exp(R1*T1)*(ppois(k12,(R1+1)*T1,log.p=FALSE)-ppois(k12,(R1+1)*T0,log.p=FALSE))/(R1+1)^(k12+1)
          +A12*R2*exp(R2*T1)*(ppois(k12,(R2+1)*T1,log.p=FALSE)-ppois(k12,(R2+1)*T0,log.p=FALSE))/(R2+1)^(k12+1)
          +((theta.a)^k12/(1+theta.a)^(k12+1))*exp(T0/theta.a)*ppois(k12,(1/theta.a + 1)*T0,log.p=FALSE)
          *(A11*exp(-R1*V)+A12*exp(-R2*V)) )

   -sum(l11)-sum(l22)-sum(l12)
}
```

```
# to obtain parameter estimates for the reparameterized IIM model (if this doesn't work, try different starting values):
IIM <- nlminb(c(isolation$par[1]/2,isolation$par[1]/2, isolation$par[2], isolation$par[3],
          (isolation$par[2]+isolation$par[3]+isolation$par[4])/4,isolation$par[4],0.5),negll.IIM,
          control=list(eval.max=10000,iter.max=10000,abs.tol= 1e-20,step.min=0.1,step.max=10),lower=rep(0,7))
# parameter estimates:
IIM.estimates <- IIM$par
# maximized loglikelihood:
IIM.maxll <- -IIM$objective
# AIC score:
IIM.AIC <- (-IIM.maxll+7)*2

# to obtain standard errors (warnings may result from nlm trying negative parameter values – for our purposes these can be ignored):
IIM2<-nlm(negll.IIM,IIM$par,hessian=TRUE)
IIM.VC<-solve(IIM2$hessian)
IIM.se<-sqrt(diag(IIM.VC))
# Note: this calculation of standard errors will not work if one or more parameters (for example, M) are estimated to be zero;
# in that case a simplified model can be fitted, removing the zero parameter(s) from the model, and estimated standard errors for the
# remaining parameters can then be computed as above under the reduced model.

# results:
# IIM.estimates = the ML estimates for (T_1, V, θ_1, θ_2, θ, θ_a, M) in the reparameterized IIM model;
# IIM.se = the estimated standard errors of these parameter estimates;
# IIM.maxll = the maximized loglikelihood for the IIM model;
# IIM.AIC = the AIC score of the IIM model.
# isolation.estimates = the ML estimates for (T, θ_1, θ_2, θ_a) in the reparameterized isolation model;
# isolation.se = the estimated standard errors of these parameter estimates;
# isolation.maxll = the maximized loglikelihood for the isolation model;
# isolation.AIC = the AIC score of the isolation model.

# to display the results:
cat("\n","IIM model:", "\n",
"ML estimate for (T_1, V, θ_1, θ_2, θ, θ_a, M):",IIM.estimates,"\n",
"estimated s.e. for (T_1, V, θ_1, θ_2, θ, θ_a, M):",IIM.se,"\n",
"maximized loglikelihood =",IIM.maxll,"\n",
"AIC score =",IIM.AIC,"\n","\n",
"isolation model:", "\n",
"ML estimate for (T, θ_1, θ_2, θ_a):",isolation.estimates,"\n",
"estimated s.e. for (T, θ_1, θ_2, θ_a):",isolation.se,"\n",
"maximized loglikelihood =",isolation.maxll,"\n",
"AIC score =",isolation.AIC,"\n")
```

### 3. R code to simulate pairwise difference data under the IIM model considered in this paper:

```
# input required: number of within- and between-species comparisons to be simulated, relative mutation rates, and parameter values:

# input numbers of simulated values required:
n11 <- # the number of loci at which two sequences from species 1 are compared (n11 ≥ 0)
n22 <- # the number of loci at which two sequences from species 2 are compared (n22 ≥ 0)
n12 <- # the number of loci at which a sequence from species 1 and a sequence from species 2 are compared (n12 ≥ 0)

# specify the relative mutation rates of the different loci:
r11 <-  # vector of length n11 containing the relative mutation rates of the loci counted in n11 (all entries of r11 must be > 0)
r22 <-  # vector of length n22 containing the relative mutation rates of the loci counted in n22 (all entries of r22 must be > 0)
r12 <-  # vector of length n12 containing the relative mutation rates of the loci counted in n12 (all entries of r12 must be > 0)
# if the same mutation rate is assumed at all loci, then input: r11 <- rep(1,n11); r22 <- rep(1,n22); r12 <- rep(1,n12)
```

# specify the values of the parameters ($\tau_1$, $\tau_0$, $c_1$, $c_2$, a, M, $\theta$) of the IIM model (see “New Approaches” and Figure 1):
# the times $\tau_1$ and $\tau_0$ (measured in units of 2N generations):

```
tau1 <- # the time since complete isolation of the two species (tau1 ≥ 0)
tau0 <- # the time since the onset of speciation (tau0 ≥ tau1)
# the relative population sizes (relative to the size of each population during the migration stage of the model):
c1 <- # the relative current size of species 1 (c1 > 0)
c2 <- # the relative current size of species 2 (c2 > 0)
a   <- # the relative size of the ancestral population (a > 0)
```

# the scaled migration and mutation rates ($M=4Nm$ and $\theta=4N\mu$):

```
M <- # twice the number of migrant gene copies per locus per generation in each direction during the migration stage of the model
        # (M > 0)
theta <- # twice the number of mutations per locus per generation in each population during the migration stage of the model,
            # averaged over all the loci considered (in n11, n22 and n12 combined)
            # (theta > 0)
```

# if the values of ($T_1$, V, $\theta_1$, $\theta_2$, $\theta$, $\theta_a$, M) are specified (see the reparameterization given by equation (4) in the main text),
# then convert these into values of the original parameters ($\tau_1$, $\tau_0$, $c_1$, $c_2$, a, M, $\theta$) as follows:

```
# tau1 <- T1/theta ; tau0 <- (T1 + V)/theta ; c1 <- theta1/theta; c2 <- theta2/theta; a <- theta.a/theta

# we scale the relative mutation rates so that their average over all the loci included in the analysis is 1:
r.average <- mean(c(r11,r22,r12))
r11 <- r11/r.average
r22 <- r22/r.average
r12 <- r12/r.average


# we first simulate the coalescence times of pairs of sequences and then superimpose mutation according to the infinite sites model:

# (i) to simulate the coalescence times of pairs of sequences from the same species:

D <- 4*M^2+1
L1 <- (2*M+1-sqrt(D))/2
L2 <- (2*M+1+sqrt(D))/2
A01 <- (L2-1)/(L2-L1)
A02 <- (1-L1)/(L2-L1)

# for pairs of sequences from species 1:
time11 <- rexp(n11,1/c1)
for (i in 1:n11){
    if (time11[i] > tau1){
        choice<-runif(1)
        if (choice < A01){ time11[i] <- tau1+rexp(1,L1)} else{time11[i] <- tau1+rexp(1,L2)}
        if (time11[i] > tau0){time11[i] <- tau0+rexp(1,1/a)}
    }
}
# result: time11 = a vector of length n11 containing the simulated coalescence times of pairs of sequences from species 1

# for pairs of sequences from species 2:
time22 <- rexp(n22,1/c2)
for (i in 1:n22){
    if (time22[i] > tau1){
        choice<-runif(1)
        if (choice < A01){ time22[i] <- tau1+rexp(1,L1)} else{time22[i] <- tau1+rexp(1,L2)}
        if (time22[i] > tau0){time22[i] <- tau0+rexp(1,1/a)}
    }
}
# result: time22 = a vector of length n22 containing the simulated coalescence times of pairs of sequences from species 2
```

# (ii) to simulate the coalescence time of a sequence from species 1 and a sequence from species 2
#       (and generate n12 such simulated values):

```
time12 <- tau1+rexp(n12,M)
for (i in 1:n12){
    repeat{
        if (time12[i] > tau0){
            time12[i] <- tau0 + rexp(1,1/a)
            break
        } else{
            time12[i] <- time12[i]+rexp(1,1+M)
            if (time12[i] > tau0){
                time12[i] <- tau0 + rexp(1,1/a)
                break
            } else{
                choice <- runif(1)
                if (choice < 1/(1+M)){break} else{time12[i] <- time12[i]+rexp(1,M)}
            }
        }
    }
}
```

# result: time12 = a vector of length n12 containing the simulated coalescence times of pairs of sequences from different species

# (iii) now superimpose mutation onto the simulated coalescence times:

```
differences11 <- rpois(n11,time11*r11*theta)
differences22 <- rpois(n22,time22*r22*theta)
differences12 <- rpois(n12,time12*r12*theta)
```

# results:
# differences11: contains the simulated numbers of differences between 2 sequences from species 1, at n11 independent loci
# differences22: contains the simulated numbers of differences between 2 sequences from species 2, at n22 independent loci
# differences12: contains the simulated numbers of differences between a sequence from species 1 and a sequence from species 2,
#                         at n12 independent loci

# **Note:**
# - to simulate coalescence times or numbers of pairwise differences under a **symmetric IM model**: input tau1 <- 0;
# - to simulate coalescence times or numbers of pairwise differences under a **complete isolation model**: input tau0 <- tau1; M <- 1
#                                                                                                                     (or any other value of M > 0);
# alternatively a simplified version of the above code tailored to these reduced models is available from the author upon request.

**References**


Takahata N, Satta Y, Klein J. 1995. Divergence time and population size in the lineage leading to modern humans. *Theor Popul Biol.* 48:198-221.

Wilkinson-Herbots HM. 2008. The distribution of the coalescence time and the number of pairwise nucleotide differences in the "isolation with migration" model. *Theor Popul Biol.* 73:277-288.

Wilkinson-Herbots HM. 2012. The distribution of the coalescence time and the number of pairwise nucleotide differences in a model of population divergence or speciation with an initial period of gene flow. *Theor Popul Biol.* 82:92-108.
